# Supplementary material for: ProDMPs: A Unified Perspective on Dynamic and Probabilistic Movement Primitives
Source: arXiv:2210.01531 source file (2022-10-04)
Supplement: Supplementary file 1 [file digit_replan_supplementary.tex]

\begin{figure}[h]
\captionbox{Supplementary to Fig \ref{fig:digit_replan}. Here we offer the result of all digits in the 3 steps writing task. We execute the current trajectory while refining it once new information is given. 
\label{fig:digit_replan_supplementary}}
[\textwidth]{
    \vspace{1mm}
    \begin{minipage}[t!]{0.49\linewidth}
        \includegraphics[width=\linewidth]{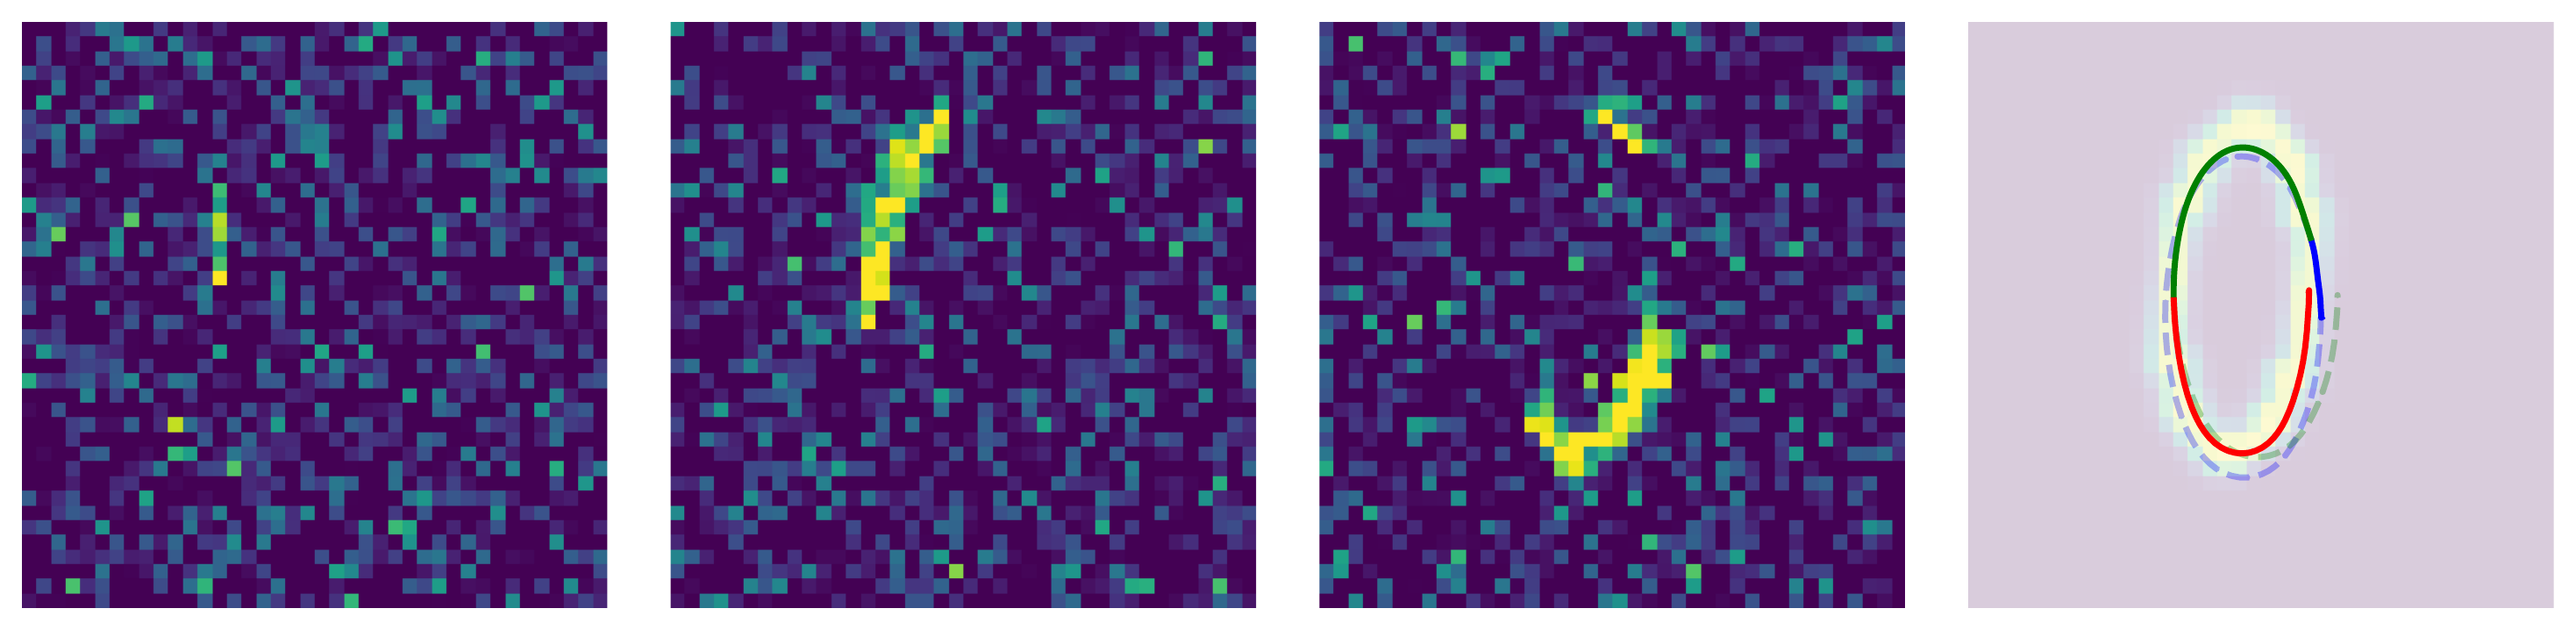}
        \label{fig:digit_replan2}
        \vspace{-4mm}
        % \subcaption[]{}
    \end{minipage}
    \hfill
    \begin{minipage}[t!]{0.49\linewidth}
        \includegraphics[width=\linewidth]{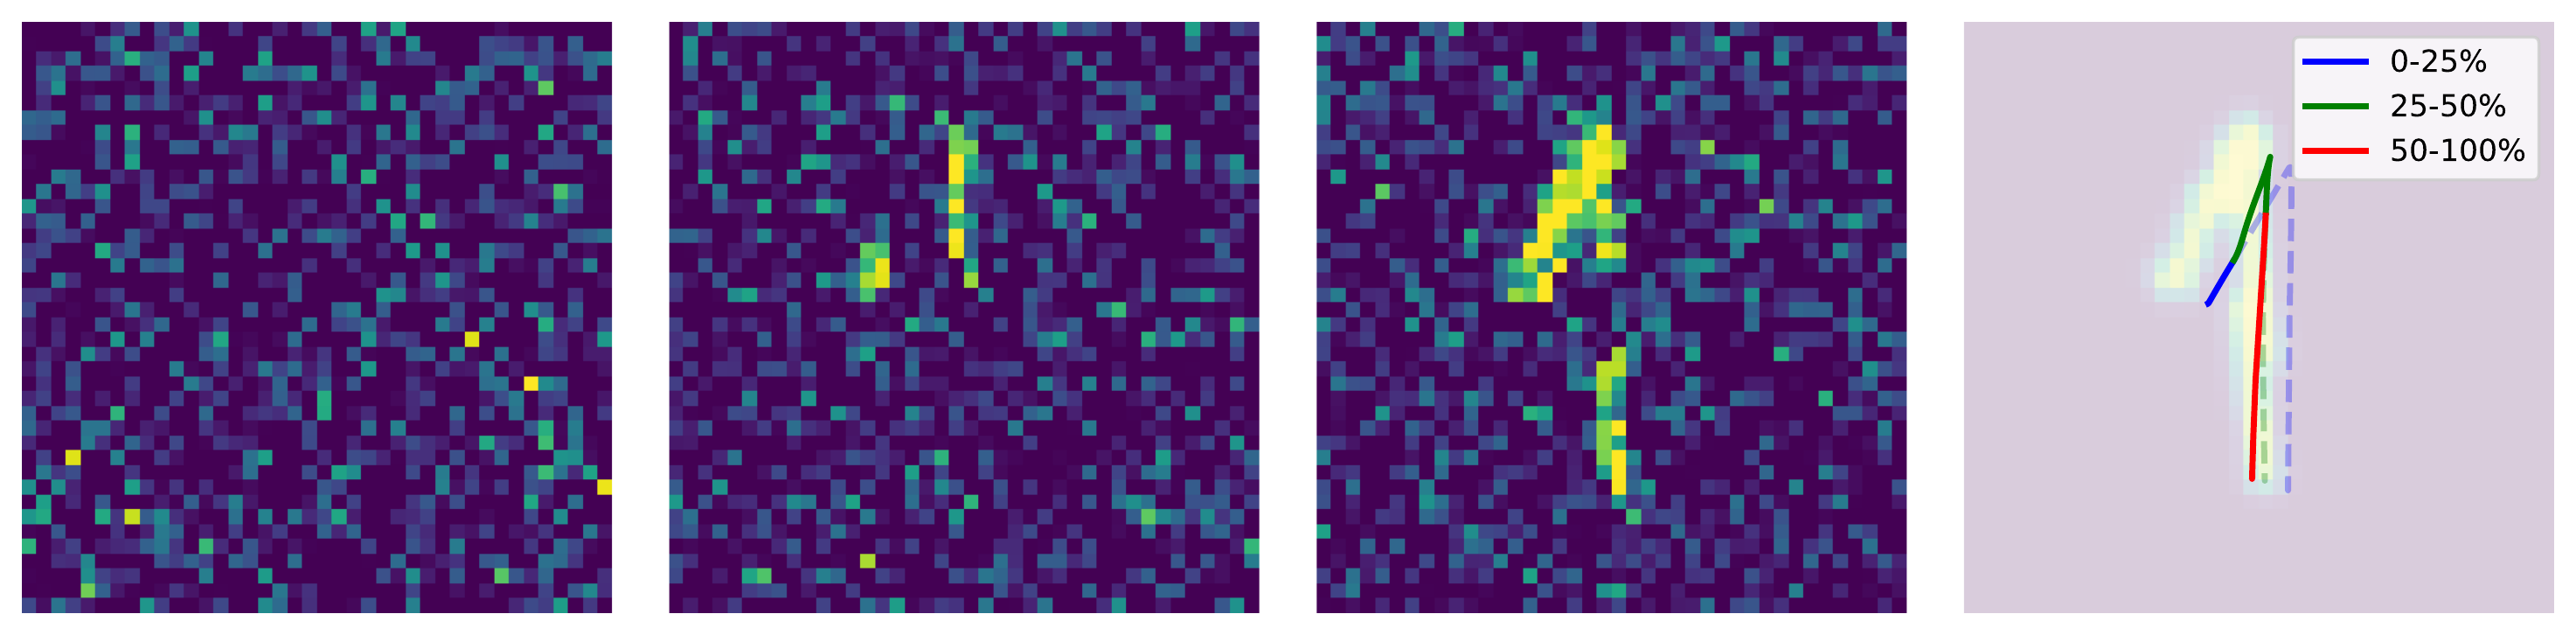}
        \label{fig:digit_replan3}
        \vspace{-4mm}
        % \subcaption[]{}
    \end{minipage}
    \begin{minipage}[t!]{0.49\linewidth}
        \includegraphics[width=\linewidth]{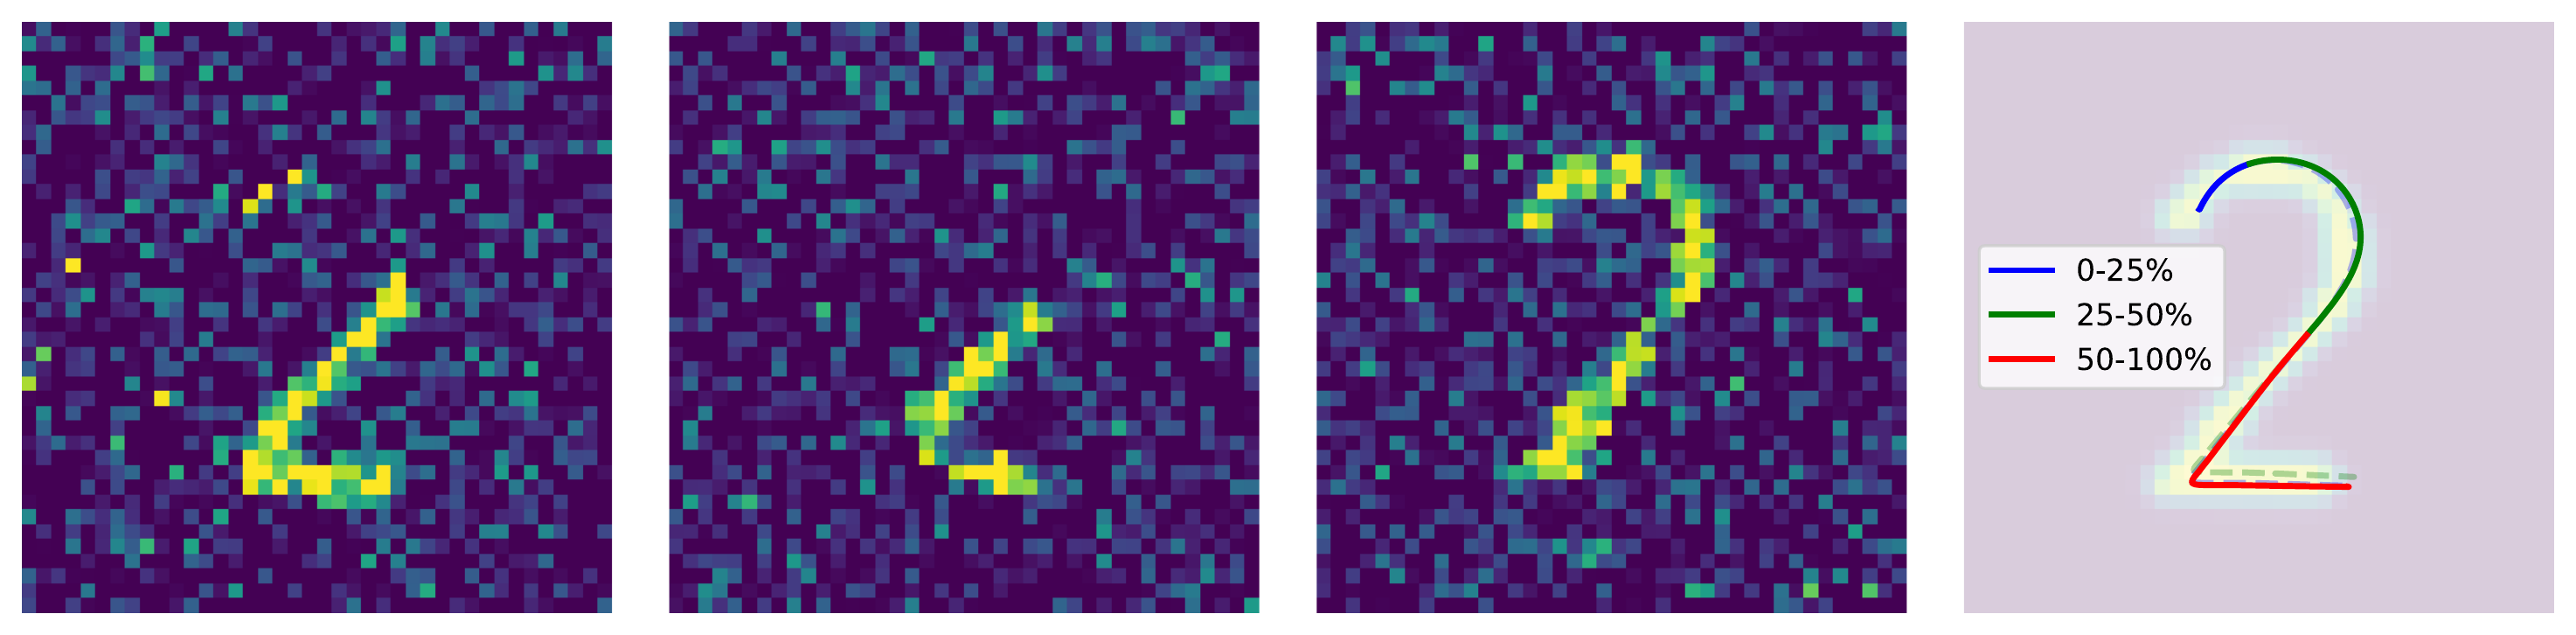}
        \label{fig:digit_replan2}
        \vspace{-4mm}
        % \subcaption[]{}
    \end{minipage}
    \hfill
    \begin{minipage}[t!]{0.49\linewidth}
        \includegraphics[width=\linewidth]{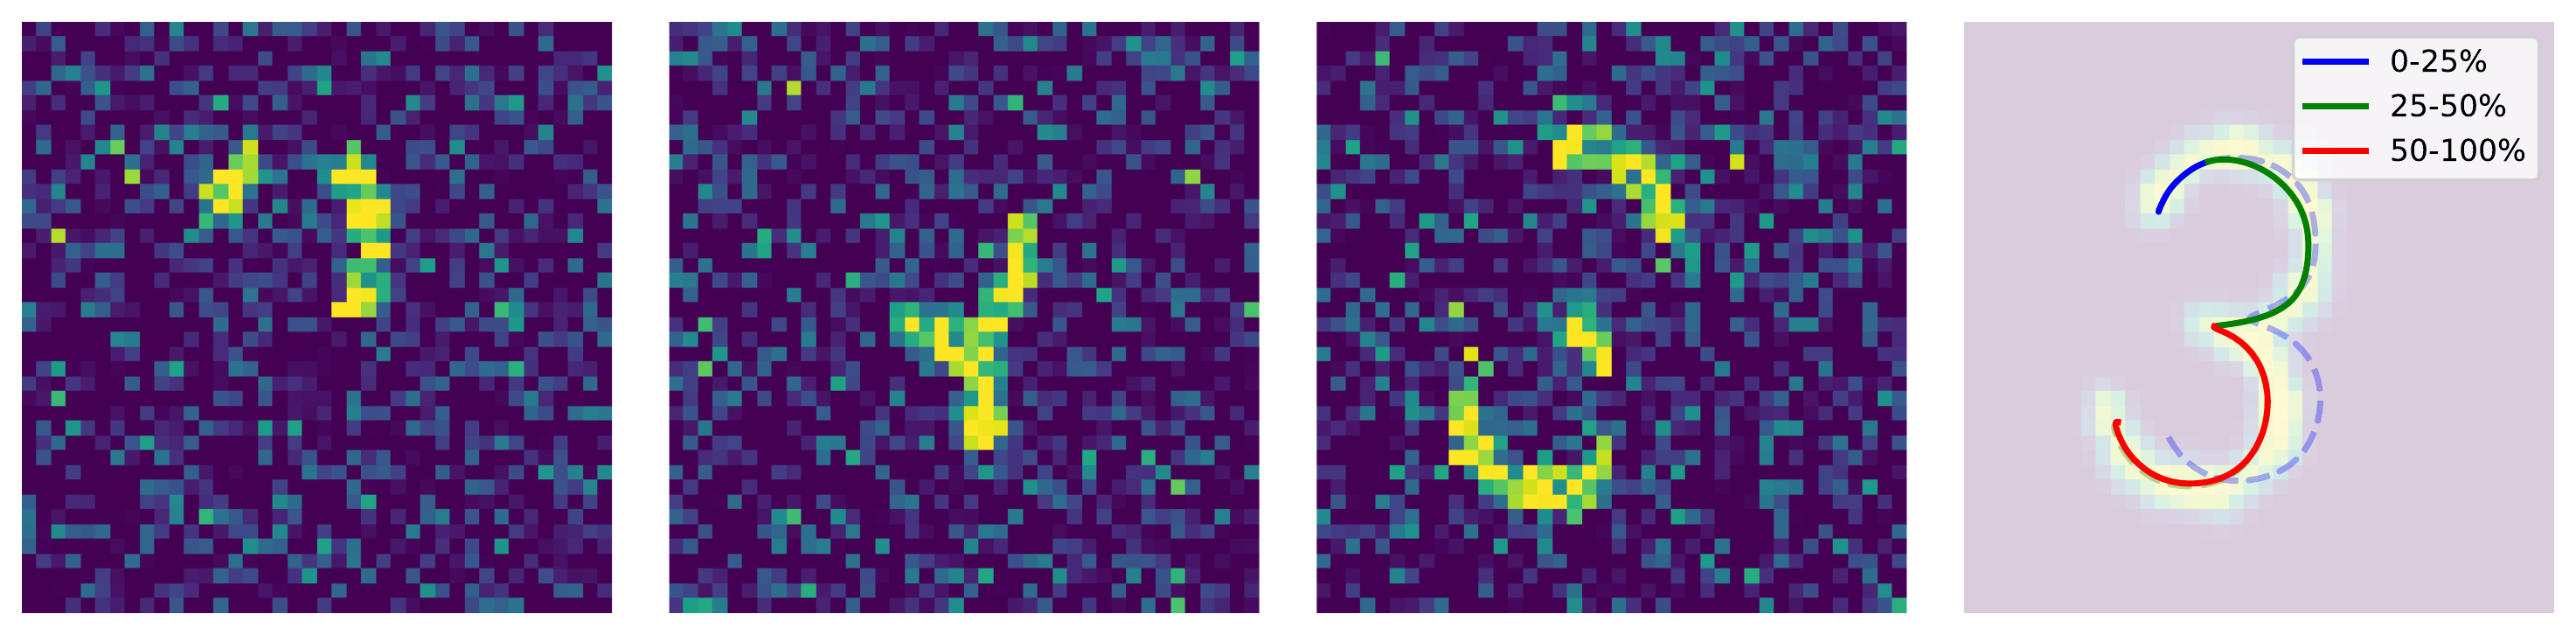}
        \label{fig:digit_replan3}
        \vspace{-4mm}
        % \subcaption[]{}
    \end{minipage}
    \begin{minipage}[t!]{0.49\linewidth}
        \includegraphics[width=\linewidth]{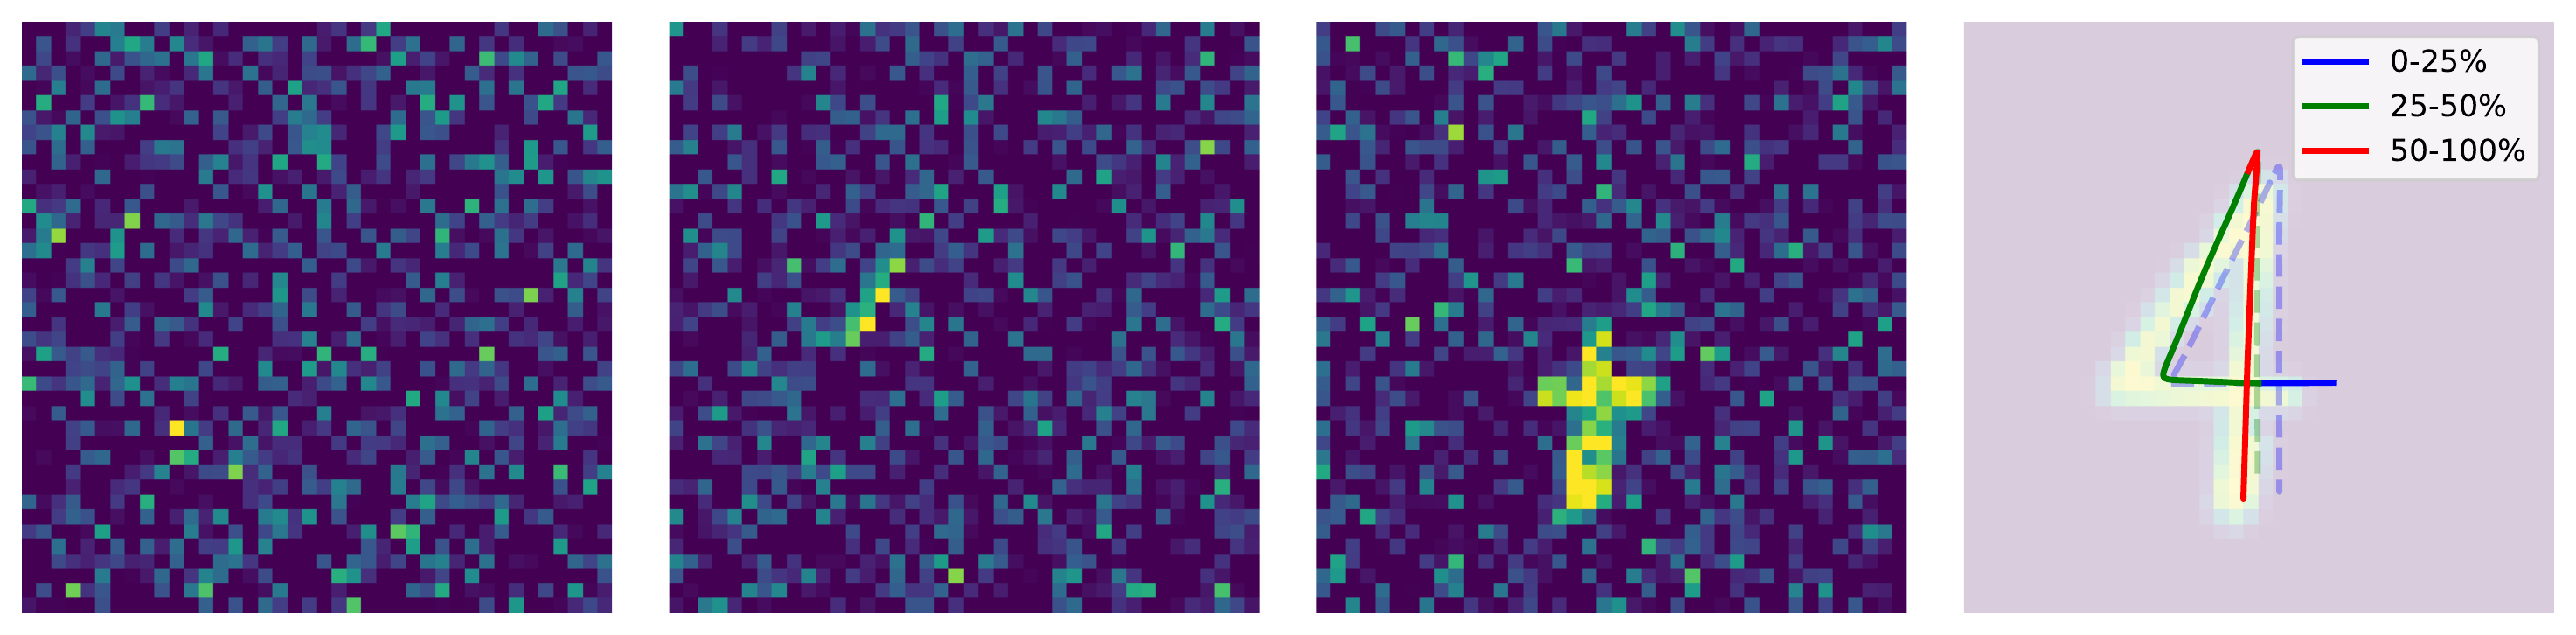}
        \label{fig:digit_replan2}
        \vspace{-4mm}
        % \subcaption[]{}
    \end{minipage}
    \hfill
    \begin{minipage}[t!]{0.49\linewidth}
        \includegraphics[width=\linewidth]{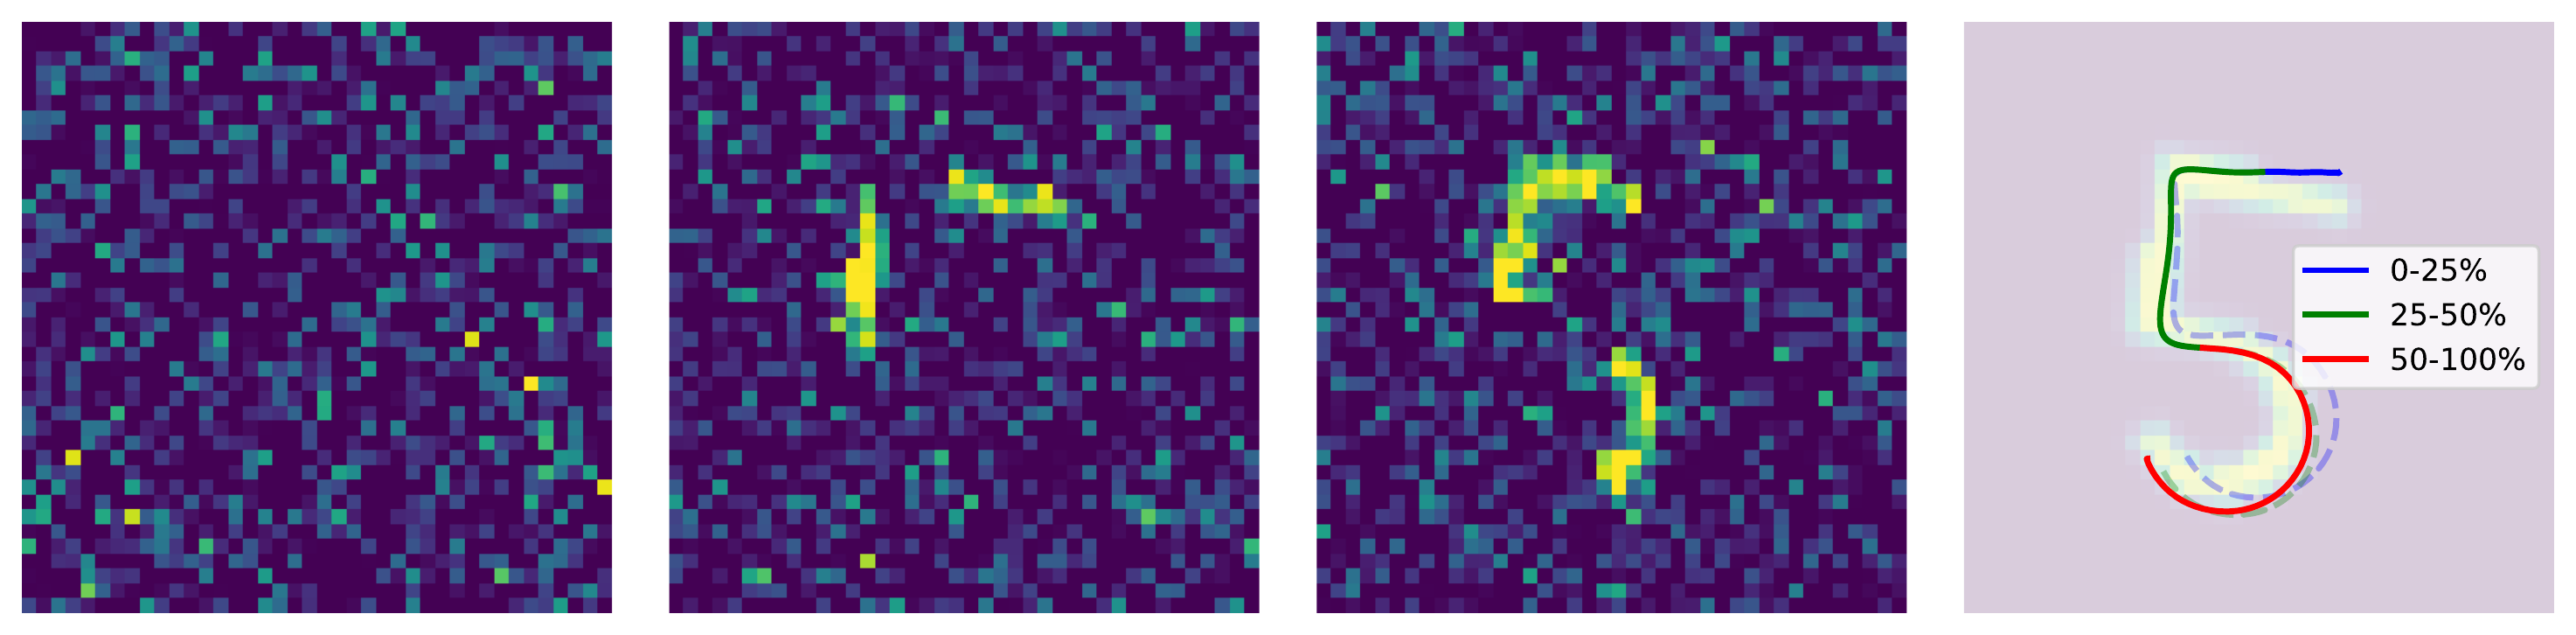}
        \label{fig:digit_replan3}
        \vspace{-4mm}
        % \subcaption[]{}
    \end{minipage}
    \begin{minipage}[t!]{0.49\linewidth}
        \includegraphics[width=\linewidth]{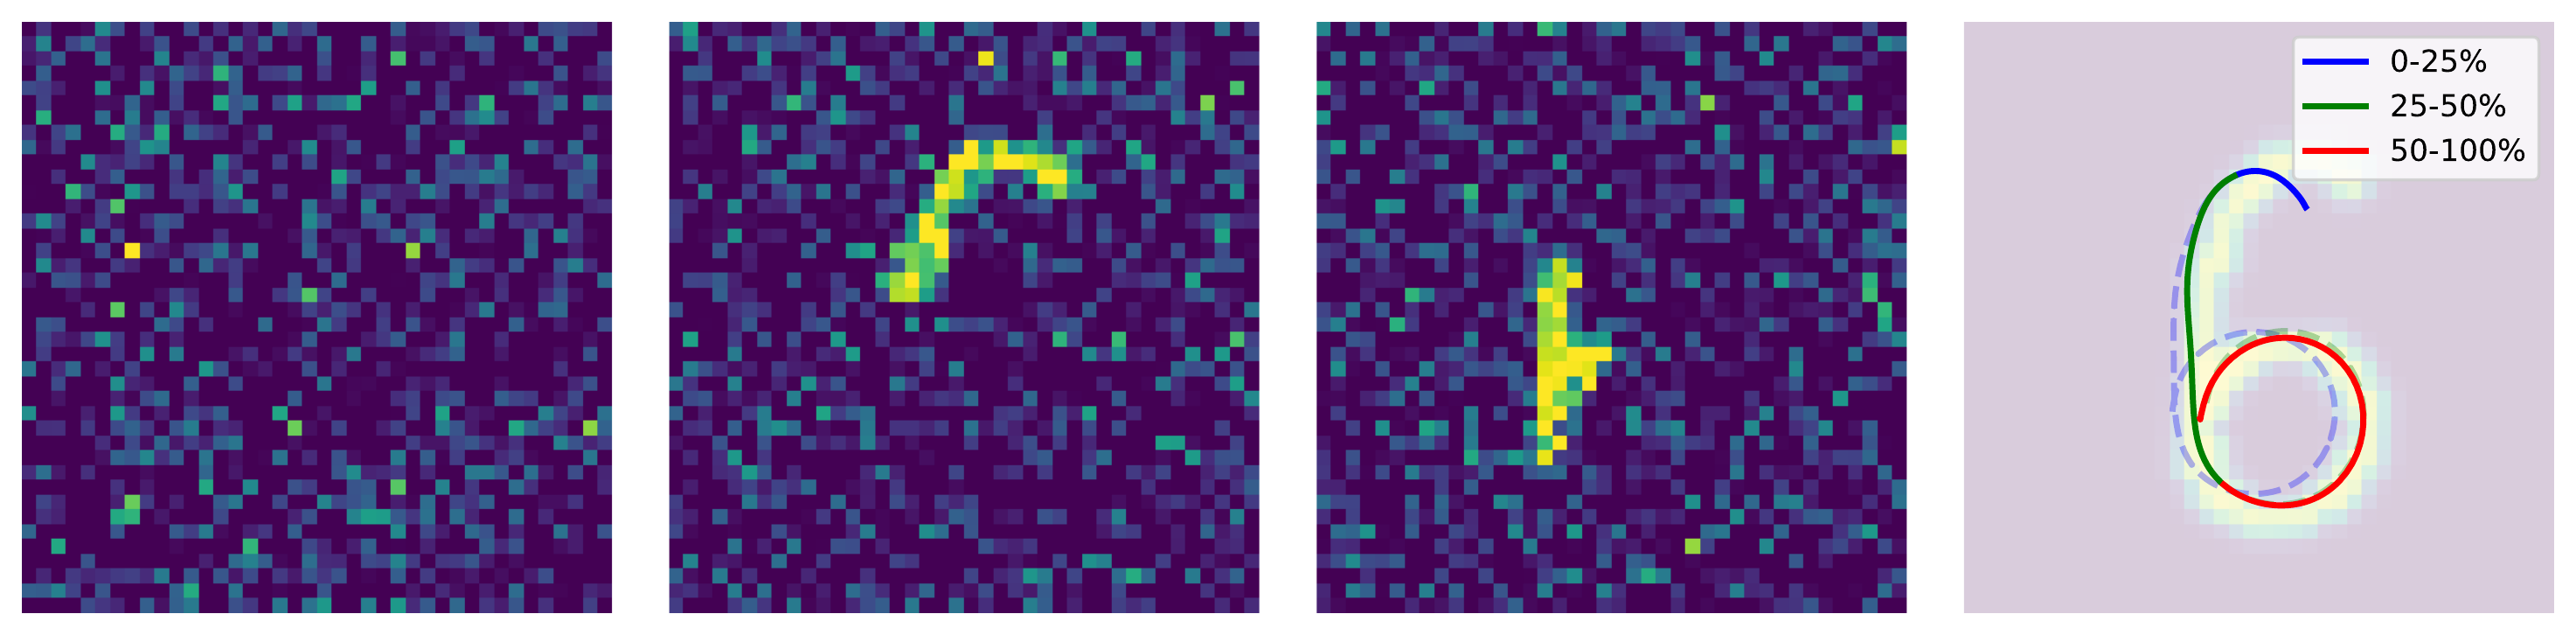}
        \label{fig:digit_replan2}
        \vspace{-4mm}
        % \subcaption[]{}
    \end{minipage}
    \hfill
    \begin{minipage}[t!]{0.49\linewidth}
        \includegraphics[width=\linewidth]{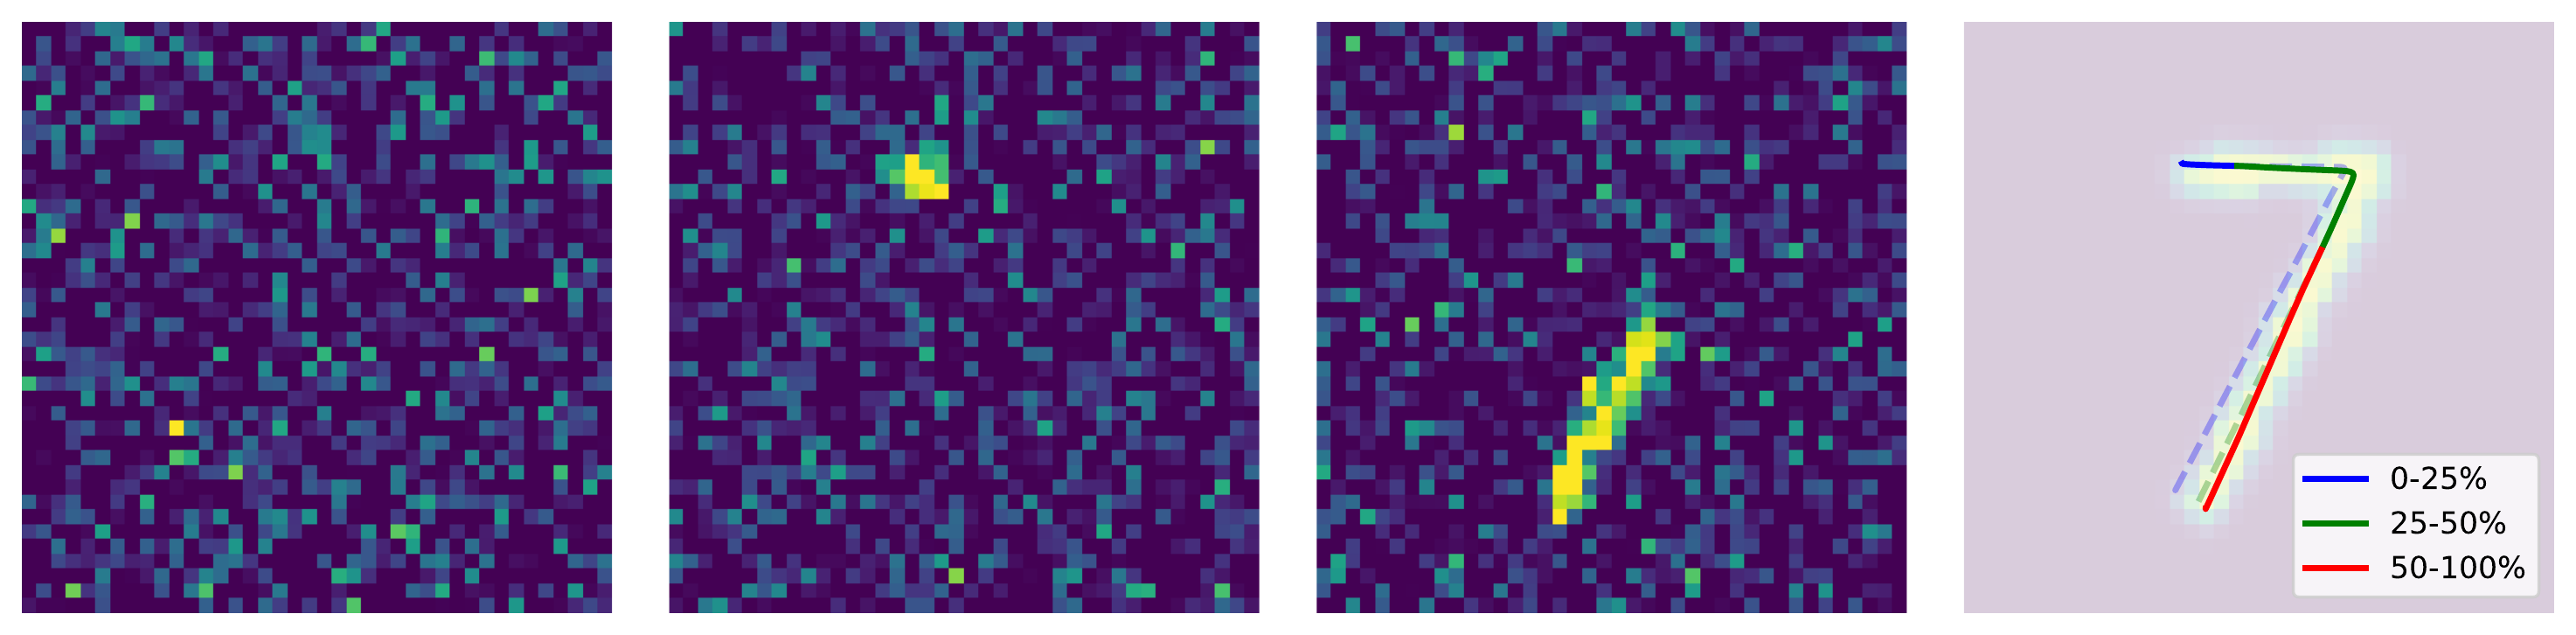}
        \label{fig:digit_replan3}
        \vspace{-4mm}
        % \subcaption[]{}
    \end{minipage}
    \begin{minipage}[t!]{0.49\linewidth}
        \includegraphics[width=\linewidth]{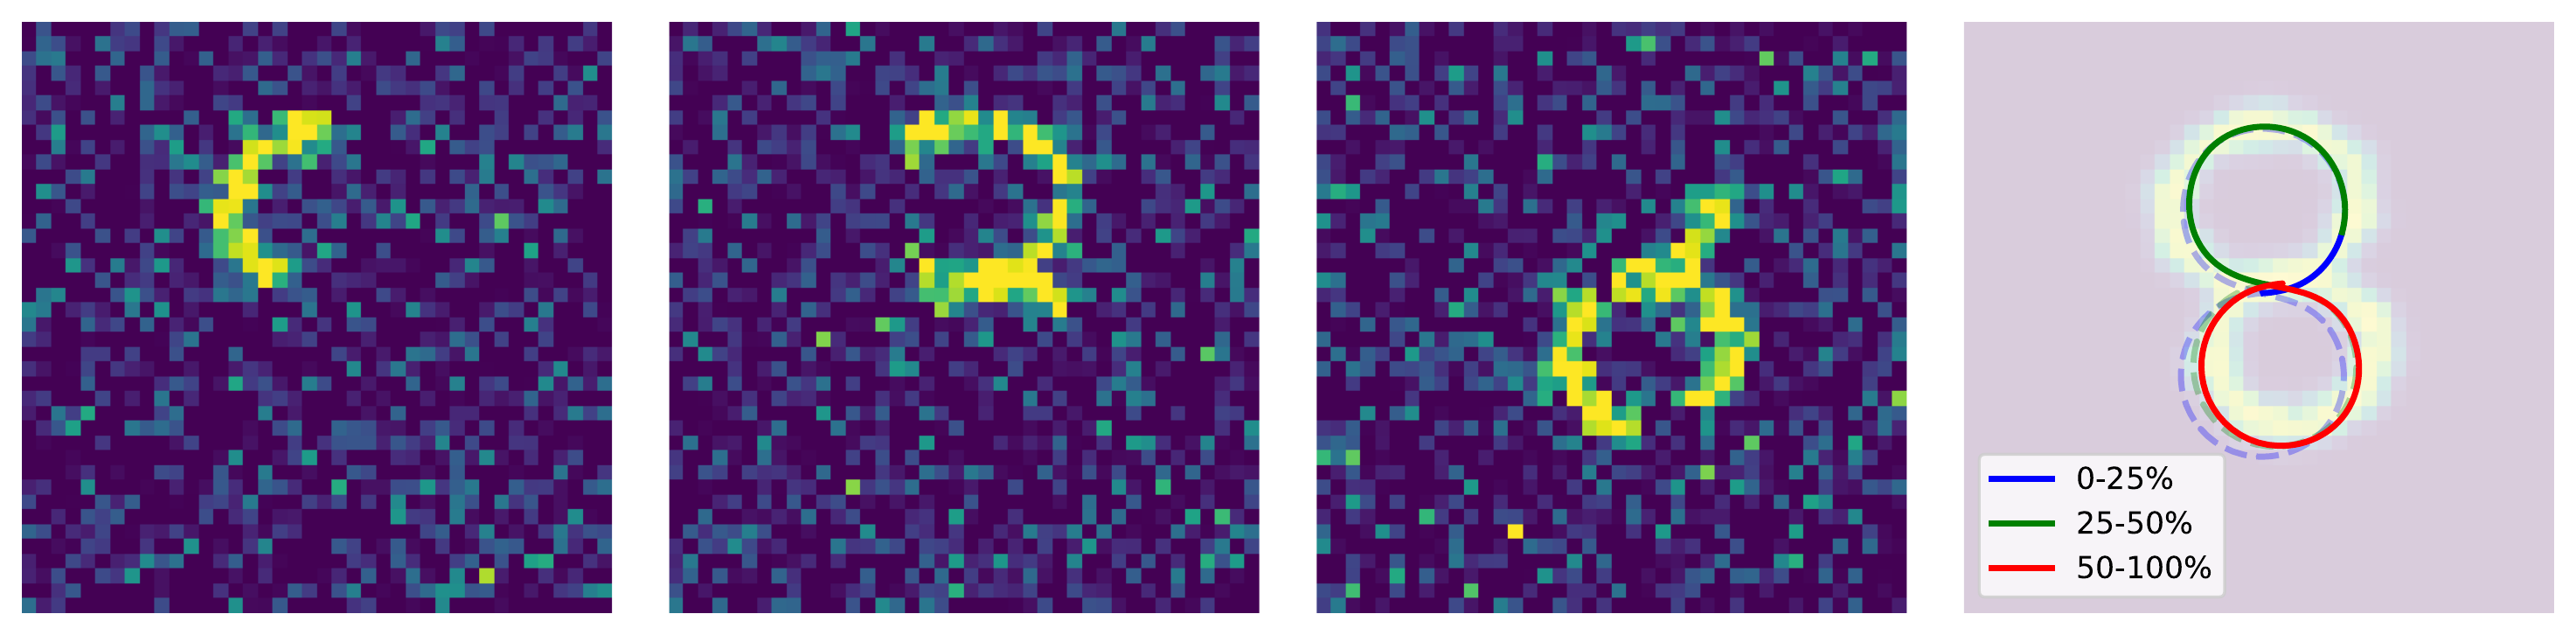}
        \label{fig:digit_replan2}
        \vspace{-4mm}
        % \subcaption[]{}
    \end{minipage}
    \hfill
    \begin{minipage}[t!]{0.49\linewidth}
        \includegraphics[width=\linewidth]{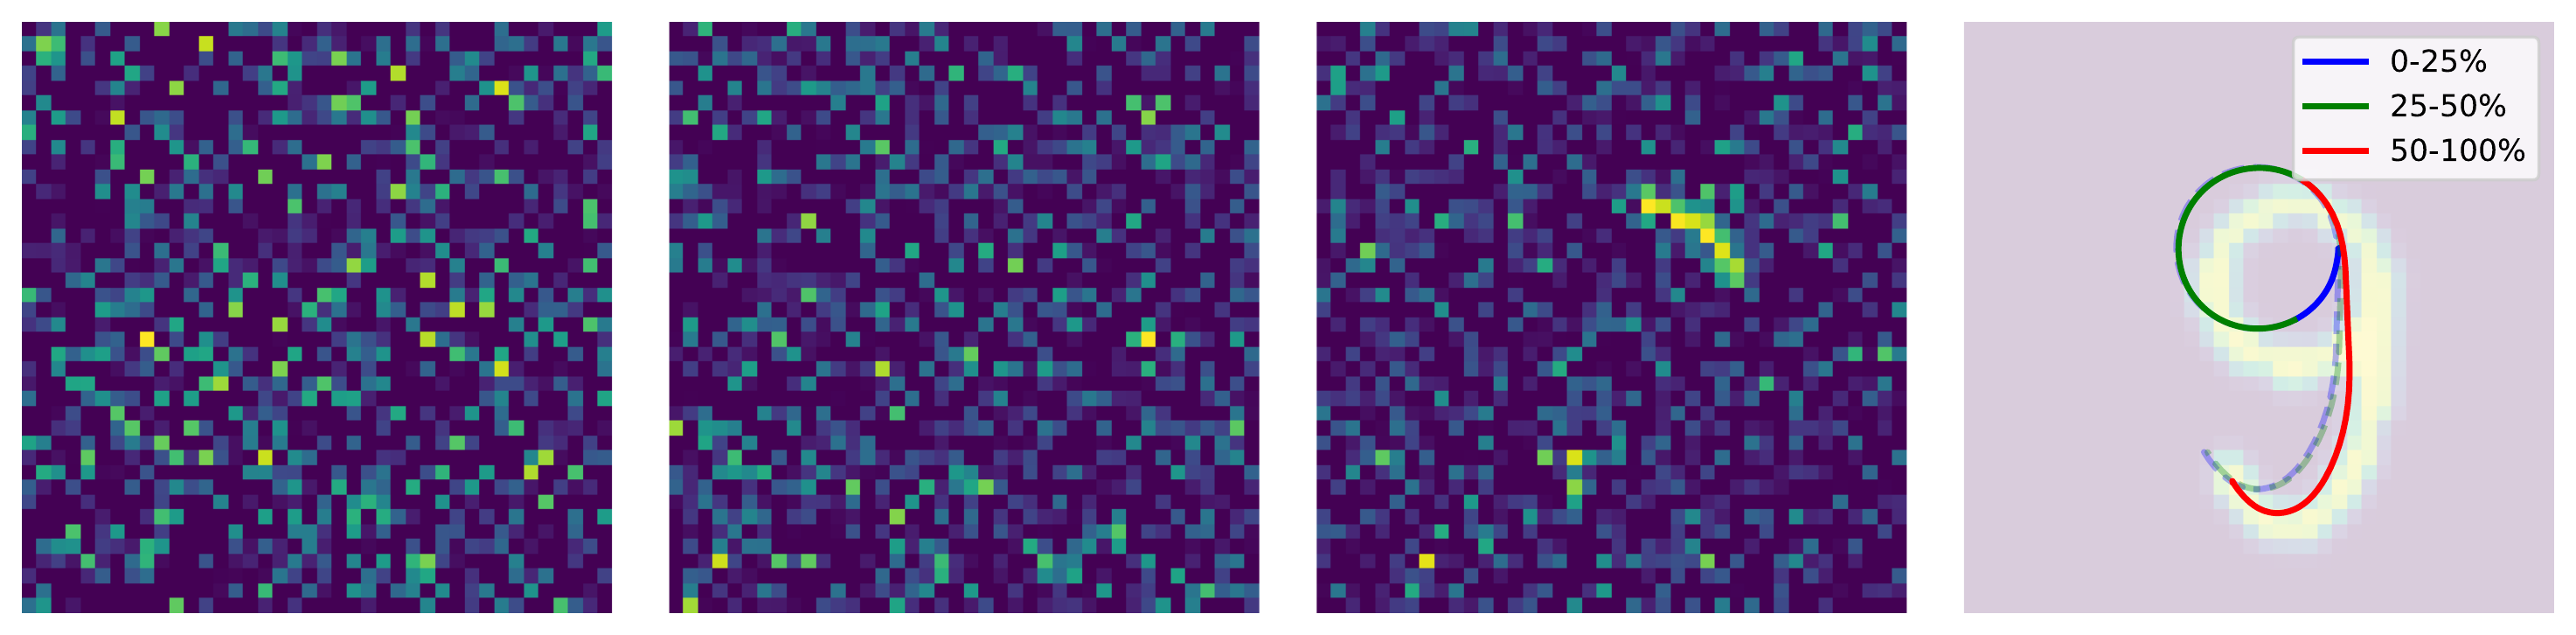}
        \label{fig:digit_replan3}
        \vspace{-4mm}
        % \subcaption[]{}
    \end{minipage}
}
\end{figure}
