# Supplementary material for: ProDMPs: A Unified Perspective on Dynamic and Probabilistic Movement Primitives
Source: arXiv:2210.01531 source file (2022-10-04)
Supplement: Supplementary file 2 [file robot_pick_additional.tex]

\begin{figure}[h]
\vspace{0.1cm}
\captionsetup[subfigure]{labelformat=empty}
\centering
\begin{minipage}[b]{0.1\textwidth}
    step 1 \\
    
    \vspace{0.12cm}
    
    step 2 \\
    
    \vspace{0.12cm}
    
    step 3 \\
    
    \vspace{0.12cm}
    
    step 4 \\
    
    \vspace{0.12cm}
\end{minipage}
\subcaptionbox{\acrshort{dof} 1}
[.22\textwidth]{
    \includegraphics[width=\linewidth]{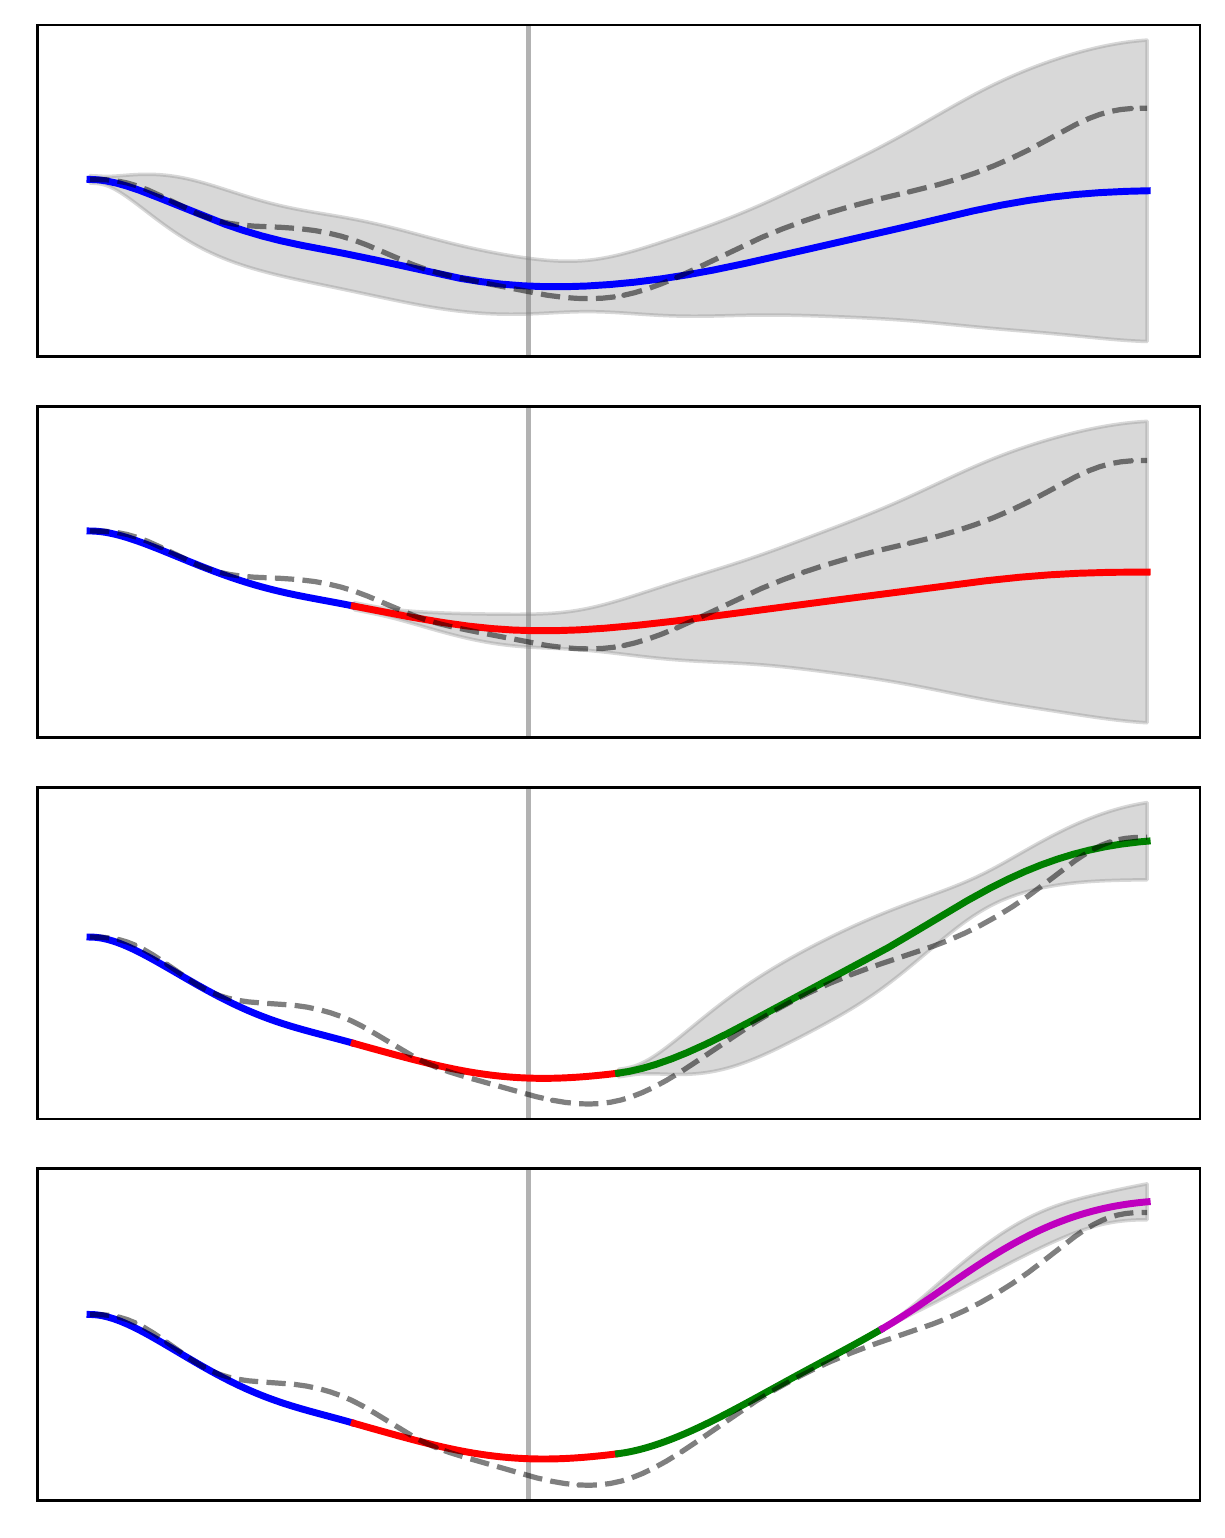}
}%
\hfill
\subcaptionbox{\acrshort{dof} 2}
[.22\textwidth]{
    \includegraphics[width=\linewidth]{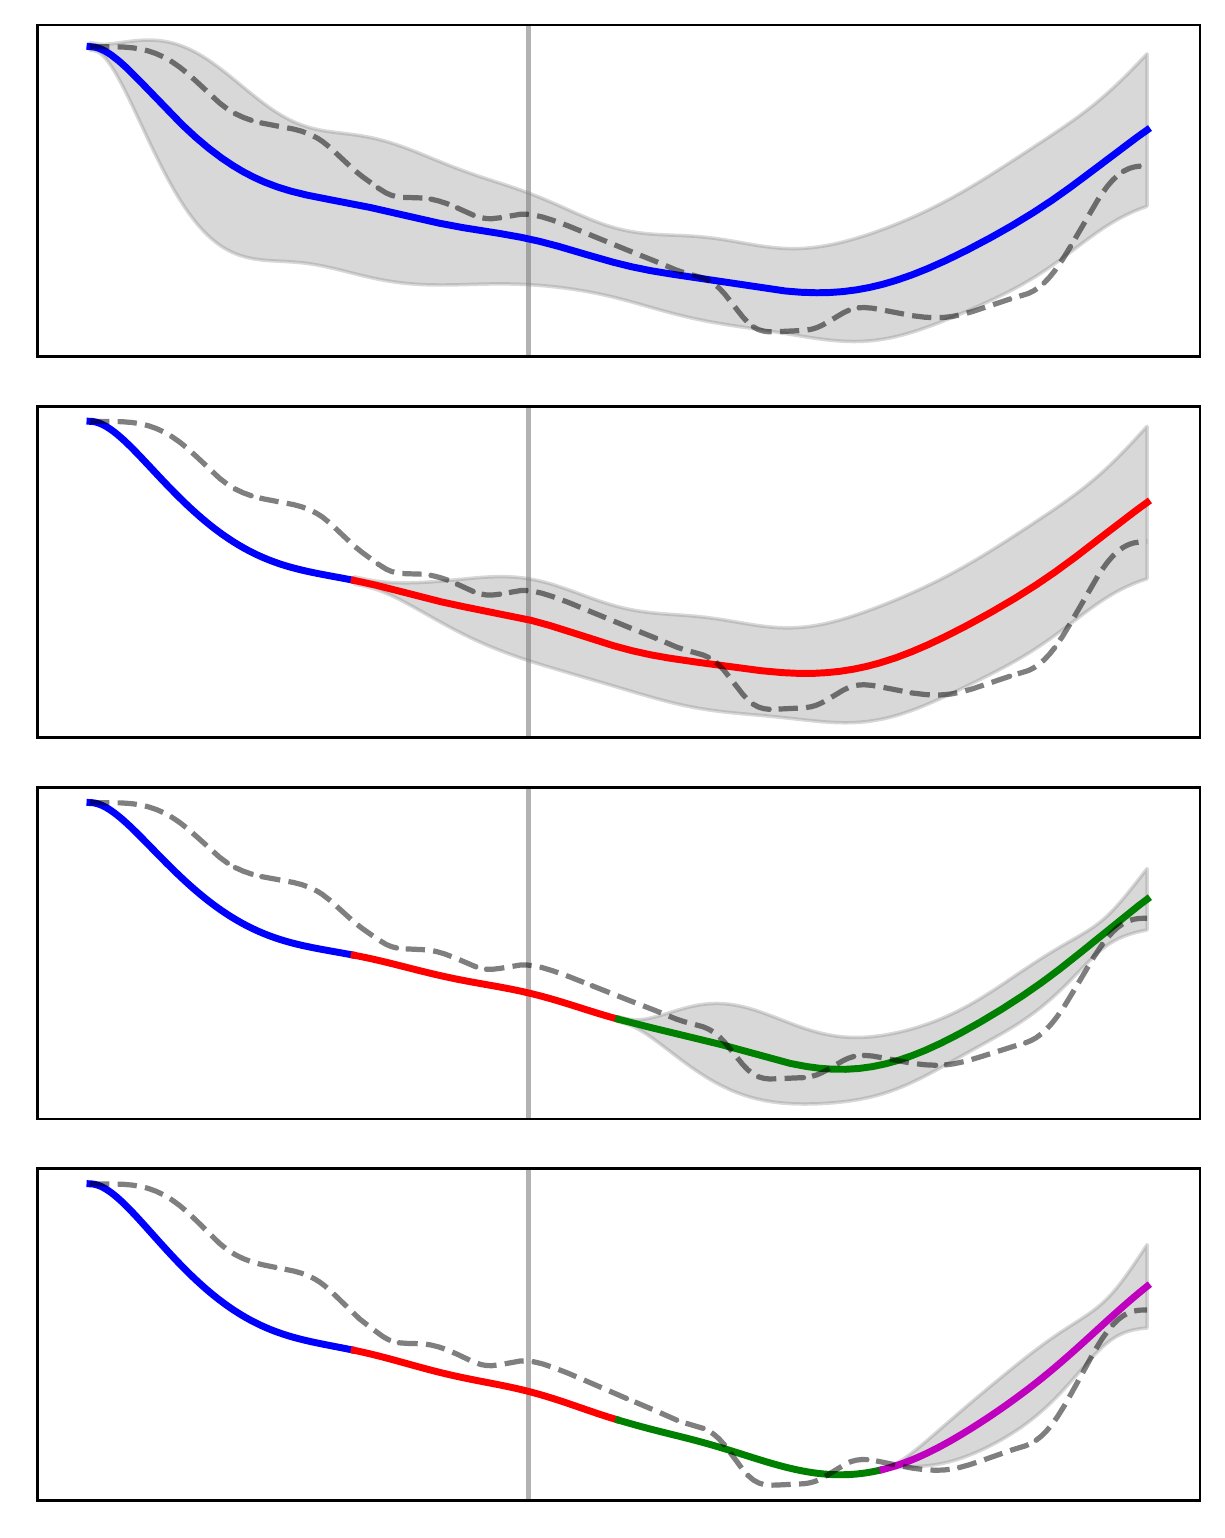}
}%
\hfill
\subcaptionbox{\acrshort{dof} 3}
[.22\textwidth]{
    \includegraphics[width=\linewidth]{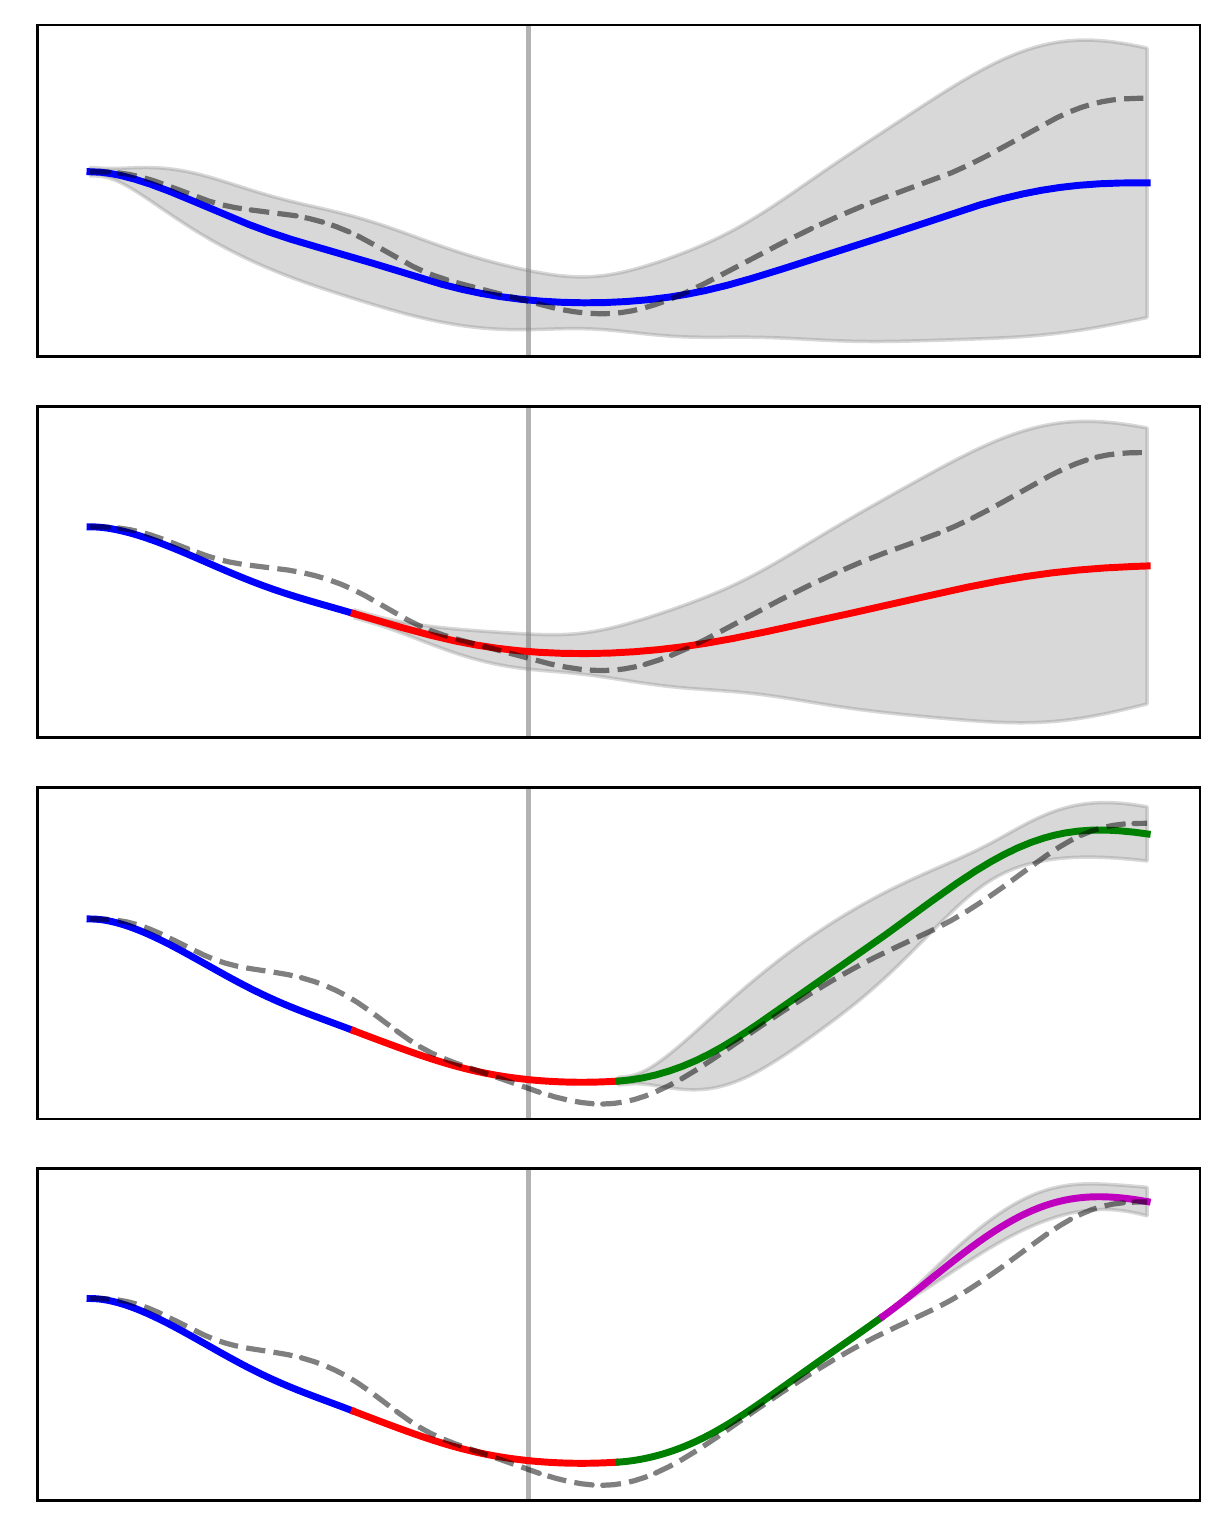}
}%
\hfill
\subcaptionbox{\acrshort{dof} 4}
[.22\textwidth]{
    \includegraphics[width=\linewidth]{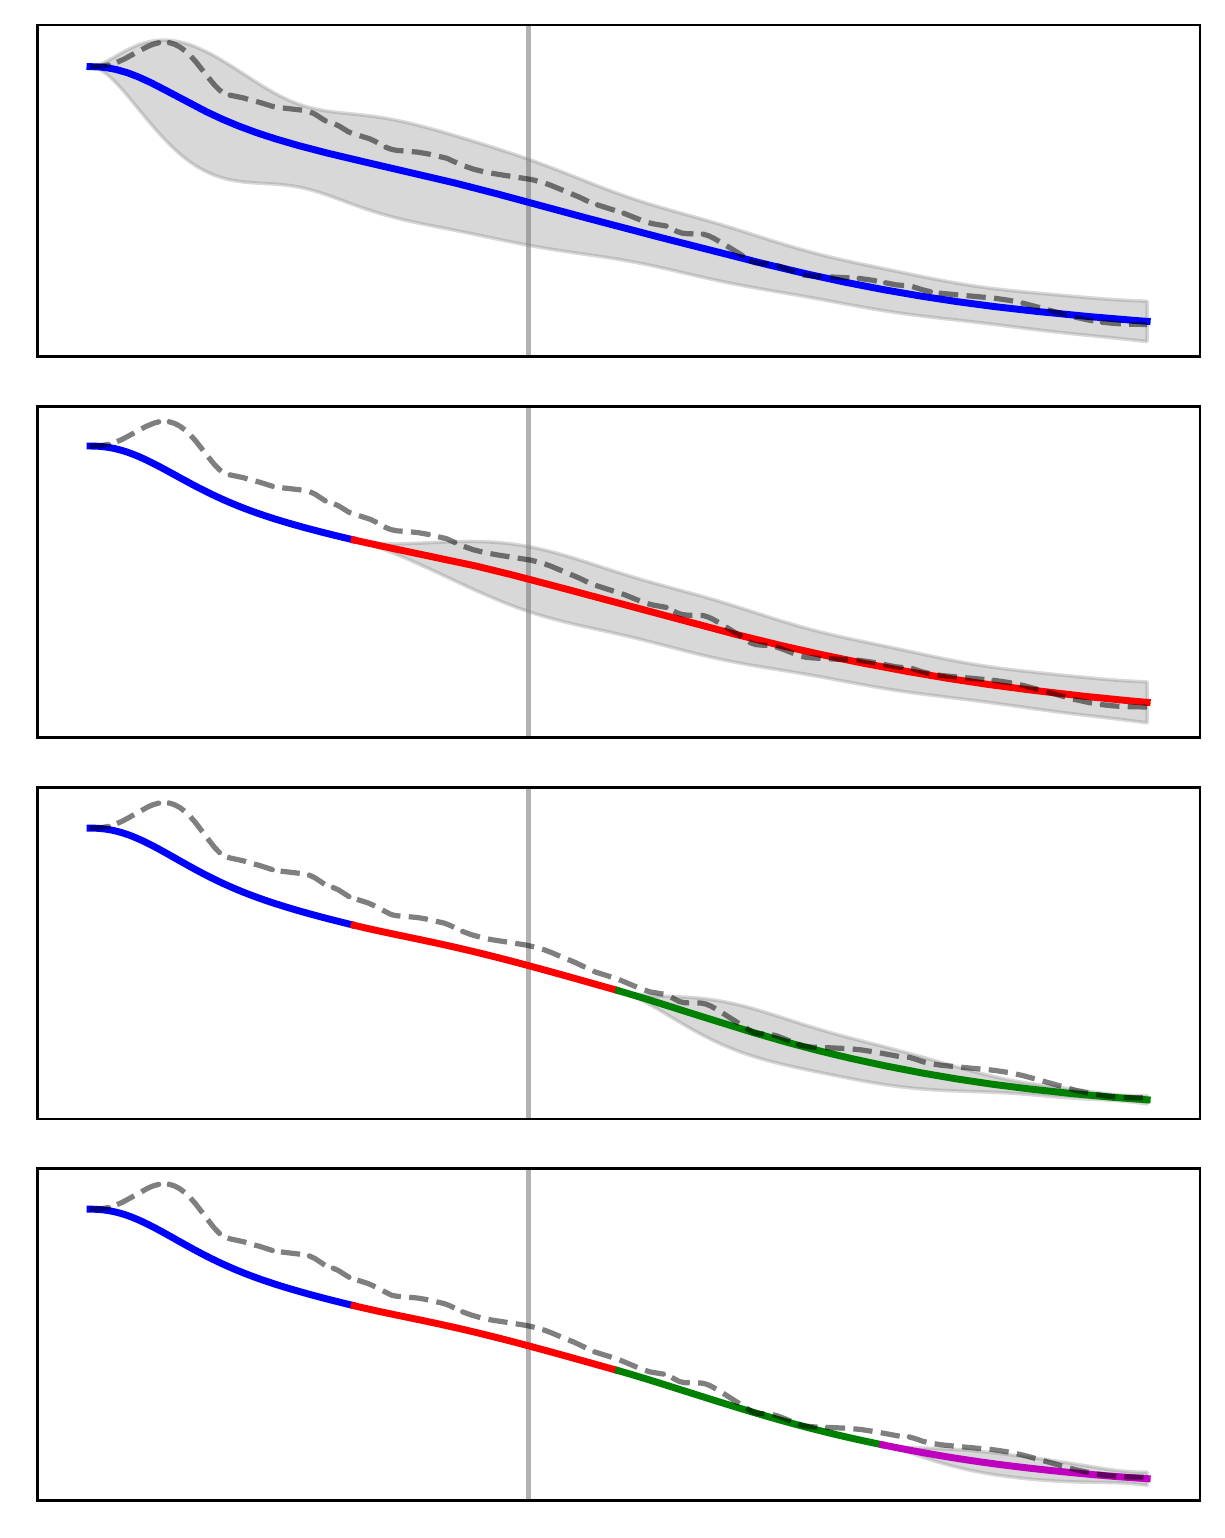}
}%
\vspace{0.2cm}
\hfill
\begin{minipage}[b]{0.1\textwidth}
    step 1 \\
    
    \vspace{0.12cm}
    
    step 2 \\
    
    \vspace{0.12cm}
    
    step 3 \\
    
    \vspace{0.12cm}
    
    step 4 \\
    
    \vspace{0.12cm}
\end{minipage}
\subcaptionbox{\acrshort{dof} 5}
[.22\textwidth]{
    \includegraphics[width=\linewidth]{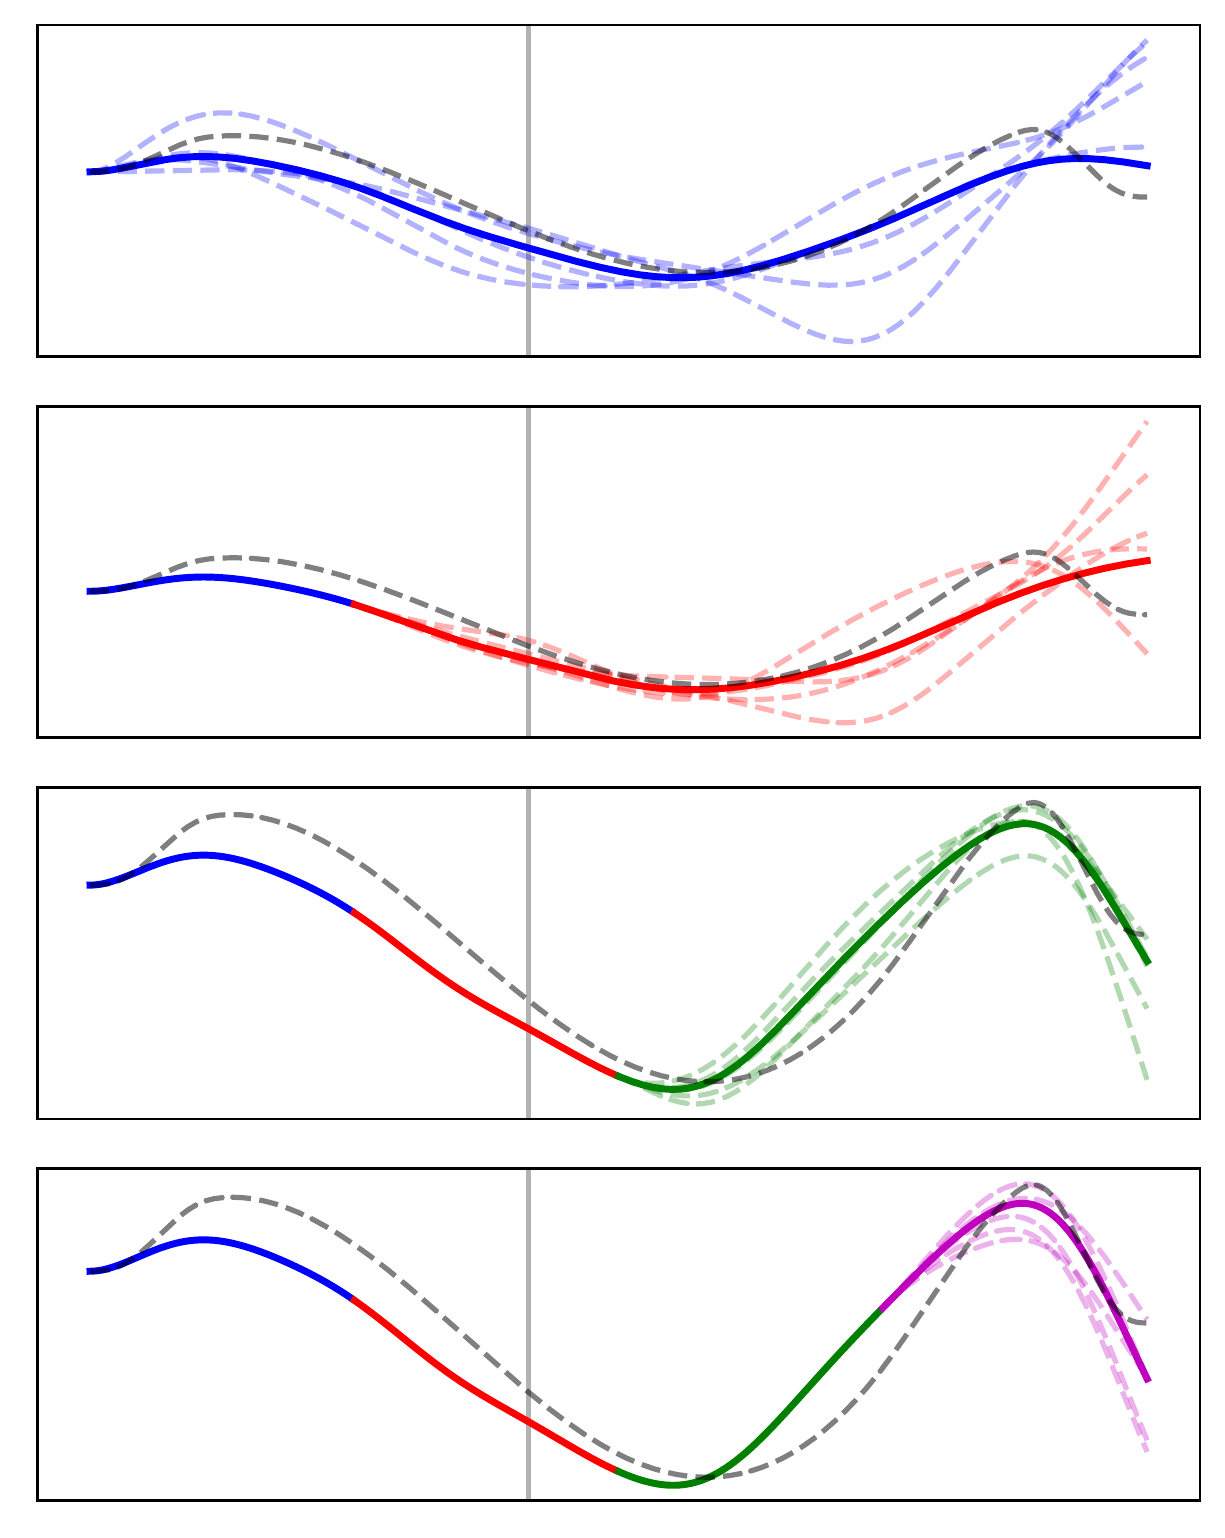}
}%
\subcaptionbox{\acrshort{dof} 6}
[.22\textwidth]{
    \includegraphics[width=\linewidth]{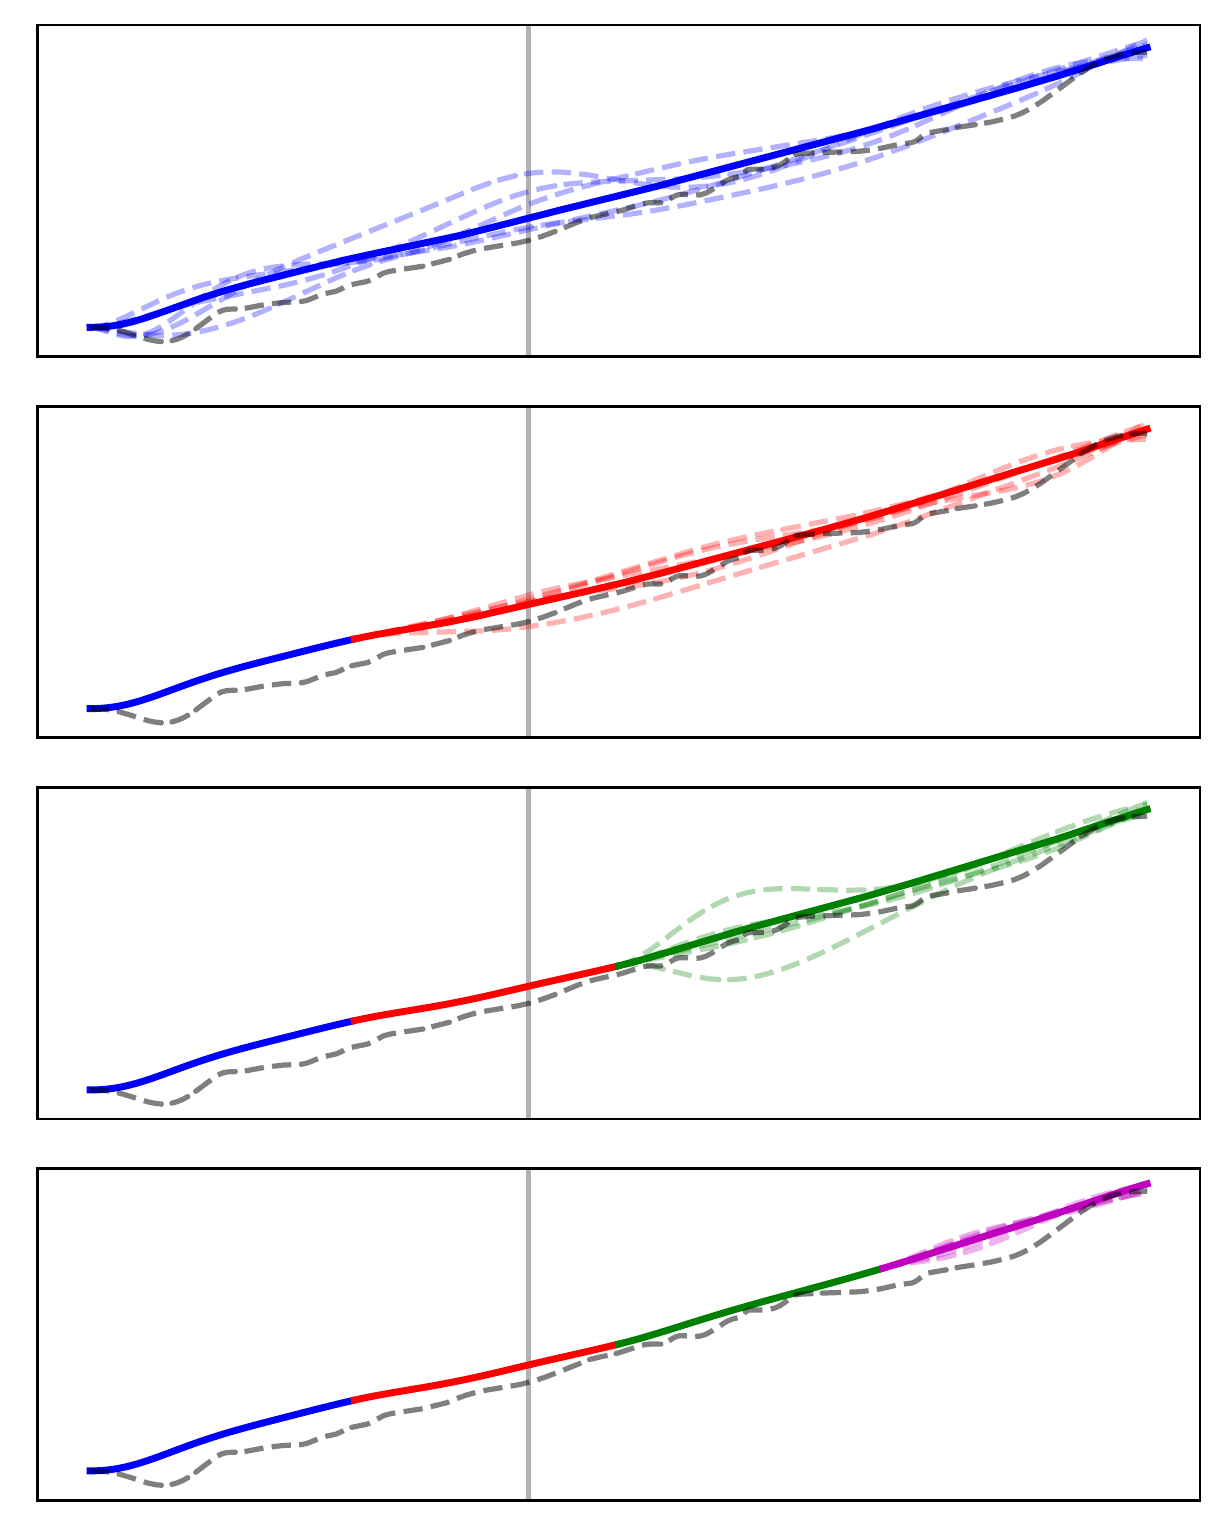}
}%
\subcaptionbox{\acrshort{dof} 7}
[.22\textwidth]{
    \includegraphics[width=\linewidth]{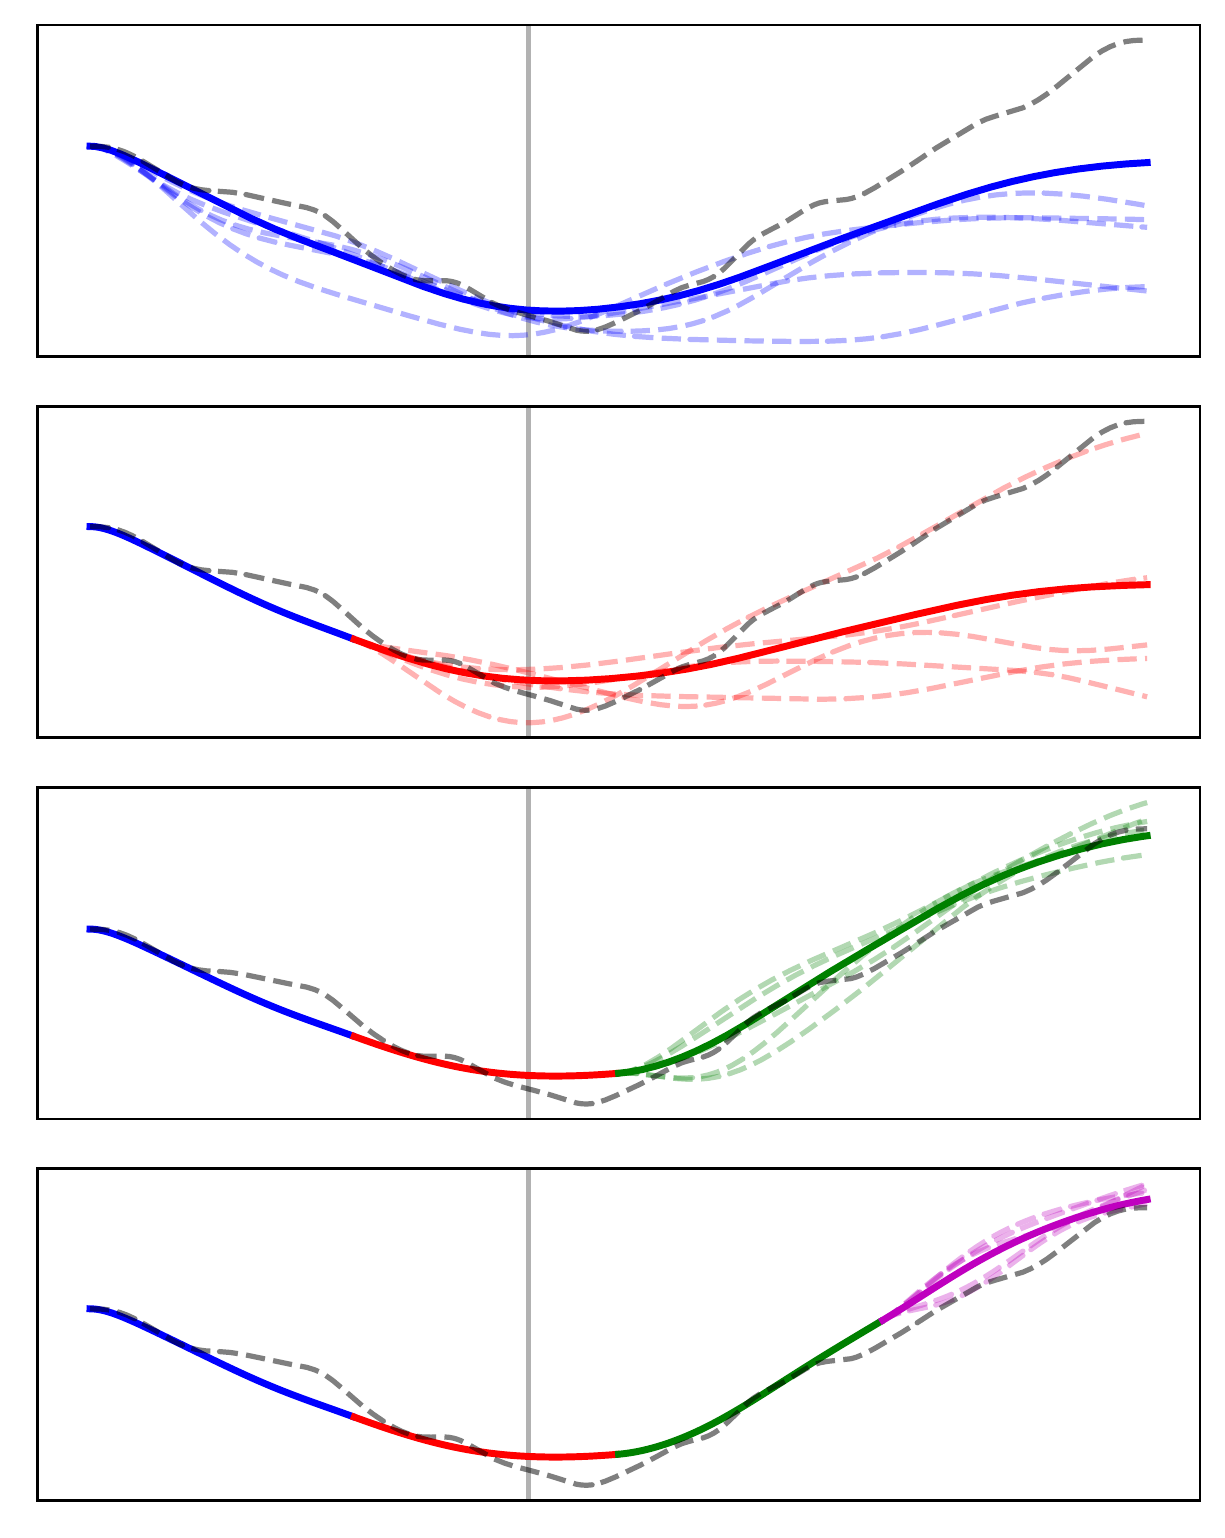}
}%
\hfill
\caption{Supplementary joint trajectories plots in 4-step replanning of the robot picking task. Here, we plot the mean and variance of the first 4 \acrshortpl{dof}, while plotting the mean and samples of the last 3 \acrshortpl{dof}. The dark gray dashed lines are human's demonstrations. The variance of the trajectory decreases drastically after the object shifted its position.}
\label{fig:robot_pick_additional}
\vspace{-0.3cm}
\end{figure}
