# Supplementary material for: ProDMPs: A Unified Perspective on Dynamic and Probabilistic Movement Primitives
Source: arXiv:2210.01531 source file (2022-10-04)
Supplement: Supplementary file 3 [file noisy_digit_additional.tex]

\begin{figure}[h]
\captionbox{More sampled trajectories, from prediction given three noisy images.\label{fig:noisy_digit_supplementary}\vspace{-0.2cm}}
[\textwidth]{
    % \subcaptionbox{}
    % [.48\textwidth]{
    %     \includegraphics[width=\linewidth]{figure/pdf/noisy_digit_additional/noisy_additional1.pdf}
    % }%
    % \subcaptionbox{}
    % [.48\textwidth]{
    %     \includegraphics[width=\linewidth]{figure/pdf/noisy_digit_additional/noisy_additional2.pdf}
    % }%
    \includegraphics[width=0.8\linewidth]{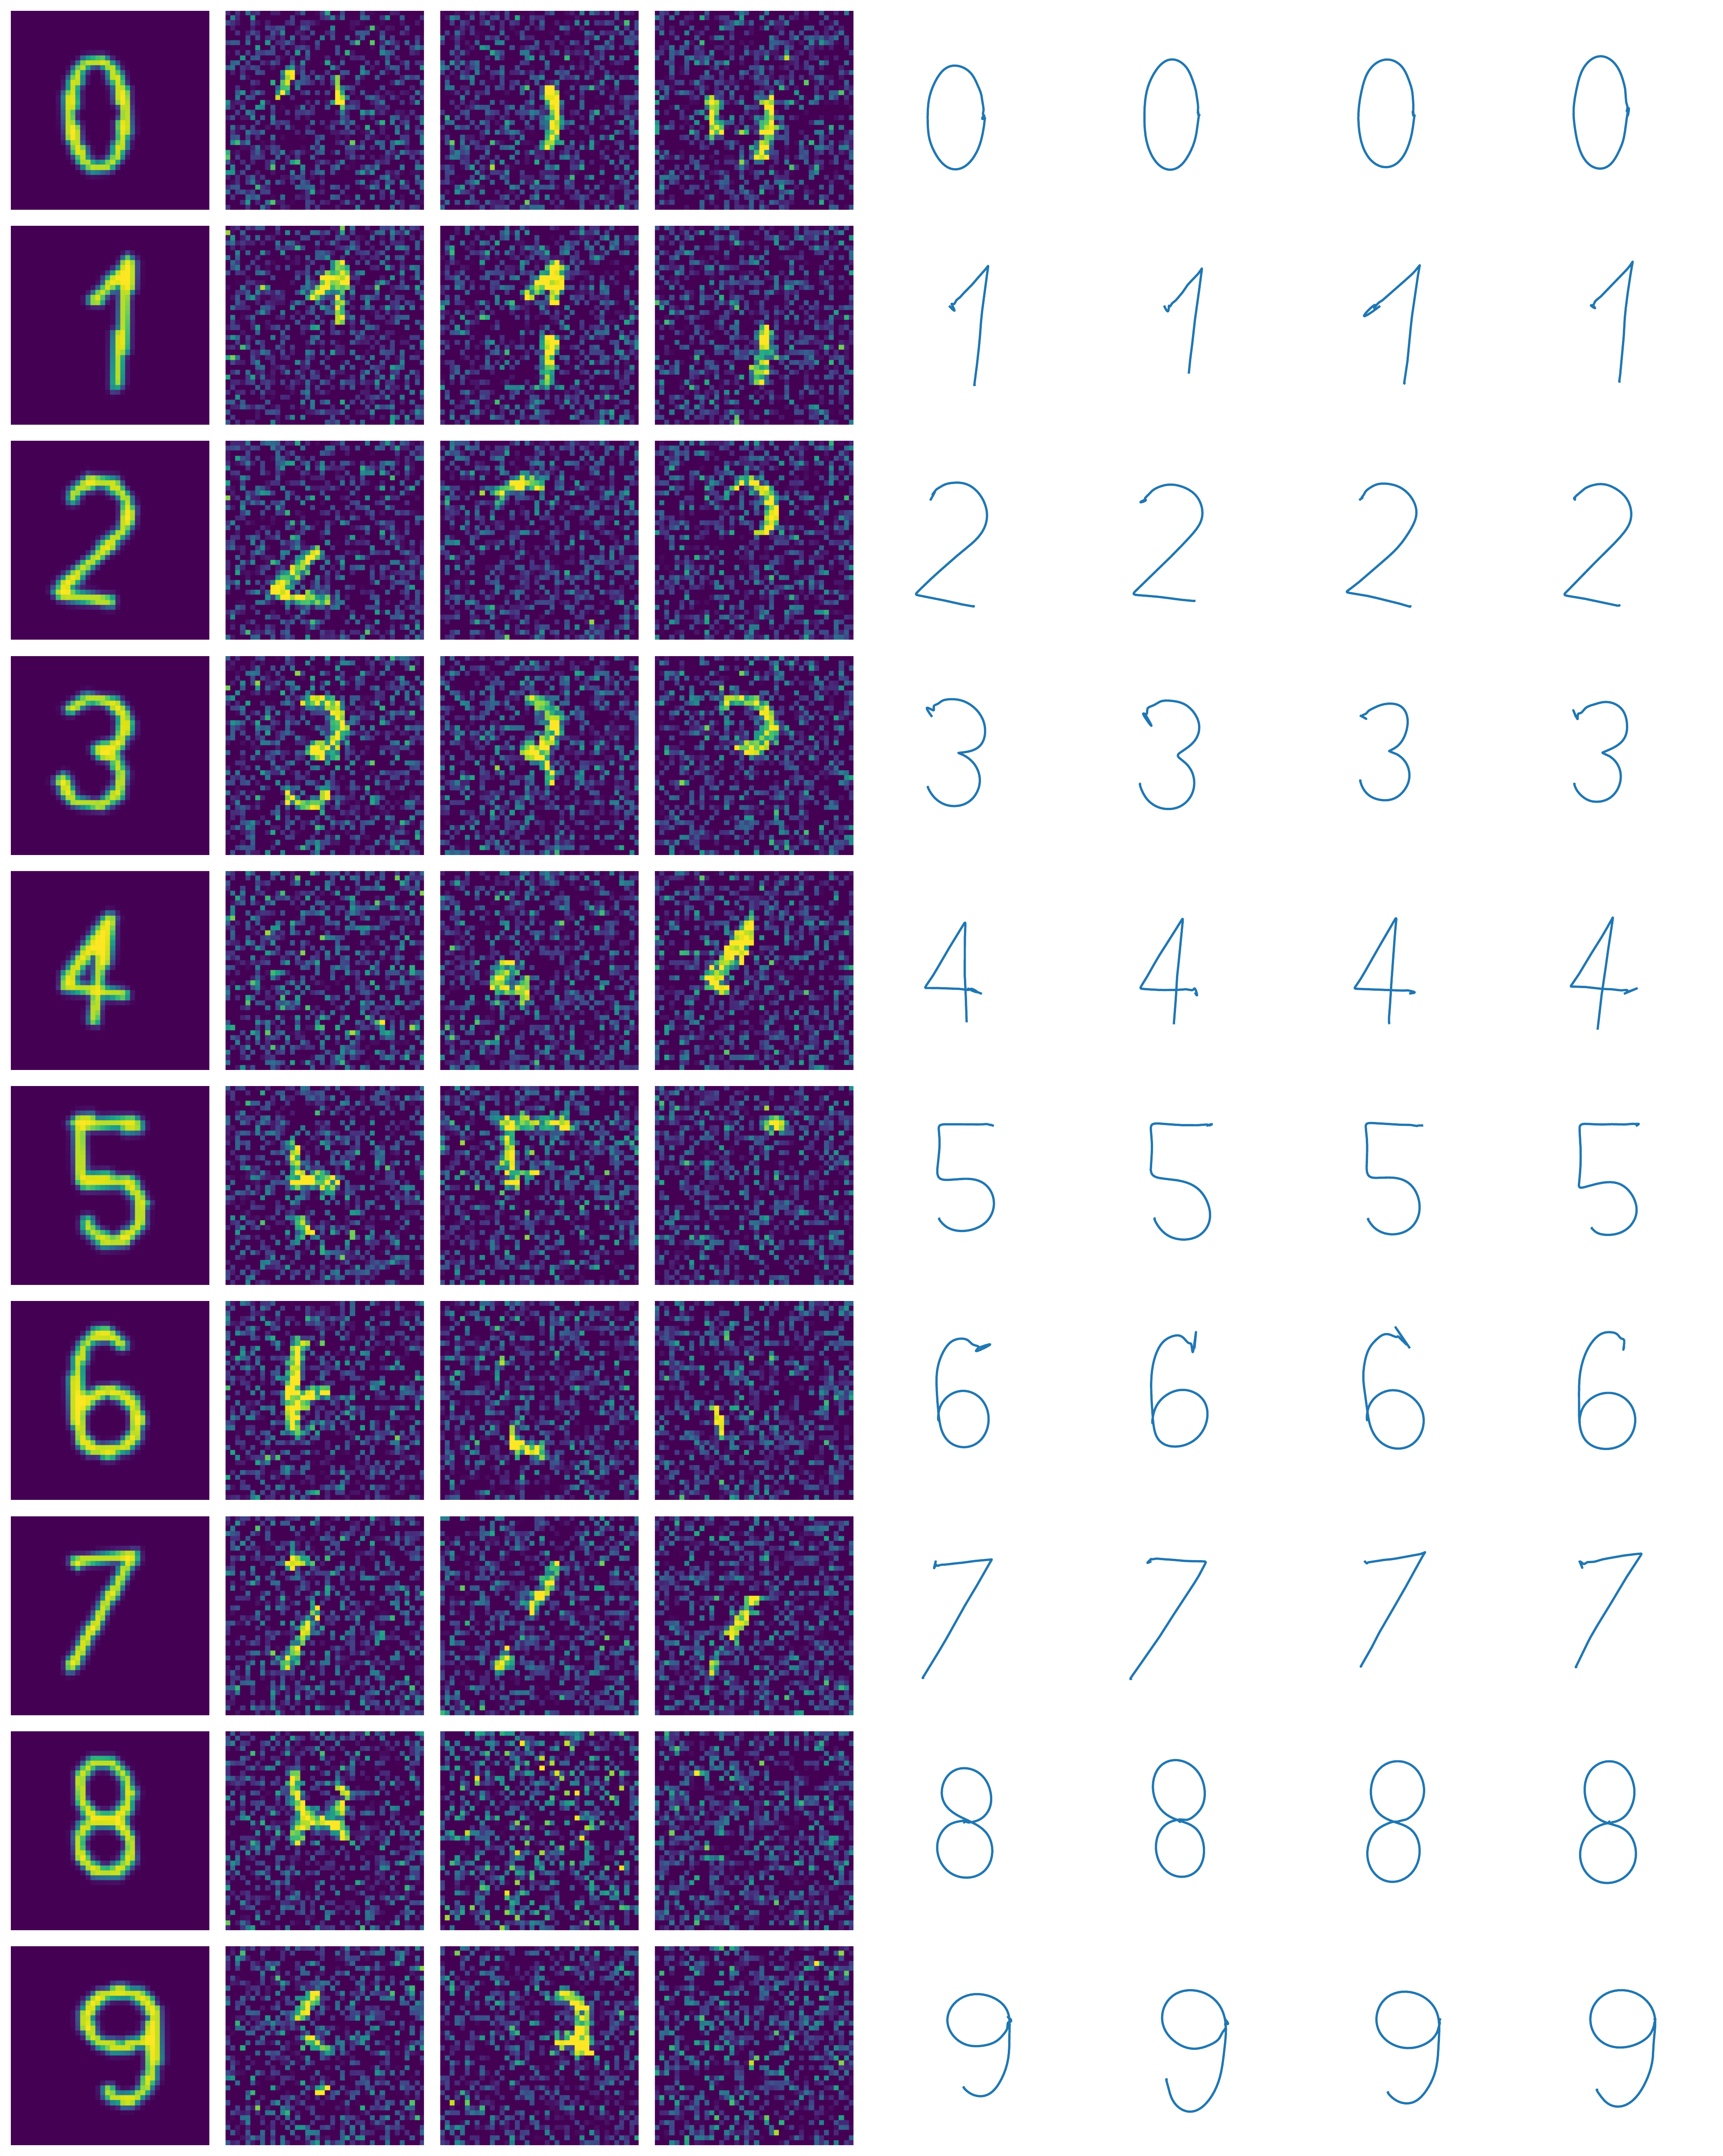}  
    }
    \vspace{-2cm}
\end{figure}
